# Supplementary material for: Guessing Smart: Biased Sampling for Efficient Black-Box Adversarial Attacks
Source: arXiv:1812.09803 source file (2019-05-05)
Supplement: Supplementary file 1 [file 99_appendix-style4.tex]

\clearpage

\begin{table*}[htp]
	\caption{The Biased Boundary Attack (targeted)}
	\begin{center}
		\begin{tabular}{c c p{1.cm} c c}
		
			% First group of 2x4
			\textbf{Original}&\textbf{Adversarial}& & \textbf{Original} & \textbf{Adversarial} \\
			European salamander & Sulphur butterfly & & & \\

			\includegraphics[width=.18\textwidth]{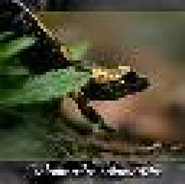} & 
			\includegraphics[width=.18\textwidth]{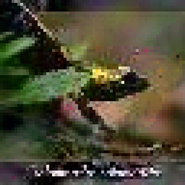} & 
			&
			\includegraphics[width=.18\textwidth]{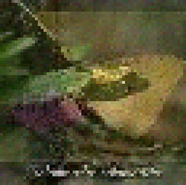} & 
			\includegraphics[width=.18\textwidth]{img/sala-1-img.png} \\

			\\
			
			\textbf{Starting point} &\textbf{Difference}& & \textbf{Starting point} & \textbf{Difference} \\
			
			\includegraphics[width=.18\textwidth]{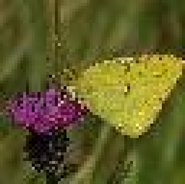} & 
			\includegraphics[width=.18\textwidth]{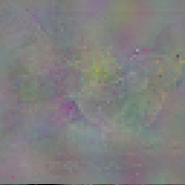} &
			&
			\includegraphics[width=.18\textwidth]{img/sala-1-img.png} & 
			\includegraphics[width=.18\textwidth]{img/sala-1-img.png} \\

			% Second group of 2x4
			\\
			\\
			\\

			\textbf{Original}&\textbf{Adversarial}& & \textbf{Original} & \textbf{Adversarial} \\
			European salamander & Sulphur butterfly & & & \\
			
			\includegraphics[width=.18\textwidth]{img/appendix-1-orig.png} & 
			\includegraphics[width=.18\textwidth]{img/appendix-1-aex.png} & 
			&
			\includegraphics[width=.18\textwidth]{img/sala-1-img.png} & 
			\includegraphics[width=.18\textwidth]{img/sala-1-img.png} \\
			
			\\
			
			\textbf{Starting point} &\textbf{Difference}& & \textbf{Starting point} & \textbf{Difference} \\
			
			\includegraphics[width=.18\textwidth]{img/appendix-1-target.png} & 
			\includegraphics[width=.18\textwidth]{img/appendix-1-diff.png} &
			&
			\includegraphics[width=.18\textwidth]{img/sala-1-img.png} & 
			\includegraphics[width=.18\textwidth]{img/sala-1-img.png} \\

			% Third group of 2x4
			\\
			\\
			\\
			
			\textbf{Original}&\textbf{Adversarial}& & \textbf{Original} & \textbf{Adversarial} \\
			European salamander & Sulphur butterfly & & & \\
			
			\includegraphics[width=.18\textwidth]{img/appendix-1-orig.png} & 
			\includegraphics[width=.18\textwidth]{img/appendix-1-aex.png} & 
			&
			\includegraphics[width=.18\textwidth]{img/sala-1-img.png} & 
			\includegraphics[width=.18\textwidth]{img/sala-1-img.png} \\
			
			\\
			
			\textbf{Starting point} &\textbf{Difference}& & \textbf{Starting point} & \textbf{Difference} \\
			
			\includegraphics[width=.18\textwidth]{img/appendix-1-target.png} & 
			\includegraphics[width=.18\textwidth]{img/appendix-1-diff.png} &
			&
			\includegraphics[width=.18\textwidth]{img/sala-1-img.png} & 
			\includegraphics[width=.18\textwidth]{img/sala-1-img.png} \\
			
		\end{tabular}	
	
		\label{tab-a3}
	\end{center}
\end{table*}
