# Supplementary material for: Guessing Smart: Biased Sampling for Efficient Black-Box Adversarial Attacks
Source: arXiv:1812.09803 source file (2019-05-05)
Supplement: Supplementary file 2 [file 999_appendix_unused.tex]

\clearpage

\begin{table*}[htp]
	\caption{The Biased Boundary Attack (targeted)}
	\begin{center}
		\begin{tabular}{c|c c c c c}
		
			\textbf{Original}&\textbf{200 Queries}& \textbf{400 Queries} & \textbf{600 Queries} & \textbf{800} & \textbf{1000}\\
				\hline 
				\\
				\includegraphics[width=.15\textwidth]{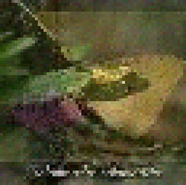} & 
				\includegraphics[width=.15\textwidth]{img/sala-1-img.png} & 
				\includegraphics[width=.15\textwidth]{img/sala-1-img.png} & 
				\includegraphics[width=.15\textwidth]{img/sala-1-img.png} & 
				\includegraphics[width=.15\textwidth]{img/sala-1-img.png} & 
				\includegraphics[width=.15\textwidth]{img/sala-1-img.png} \\

				d=1 & d=2 & d=3 & d=4 & d=5 & d=6 \\

				\includegraphics[width=.15\textwidth]{img/sala-1-img.png} & 
				\includegraphics[width=.15\textwidth]{img/sala-1-img.png} & 
				\includegraphics[width=.15\textwidth]{img/sala-1-img.png} & 
				\includegraphics[width=.15\textwidth]{img/sala-1-img.png} & 
				\includegraphics[width=.15\textwidth]{img/sala-1-img.png} & 
				\includegraphics[width=.15\textwidth]{img/sala-1-img.png} \\
			
		\end{tabular}
		\label{tab-a3}
	\end{center}
\end{table*}
